# Supplementary material for: Cross-lingual Alignment vs Joint Training: A Comparative Study and A Simple Unified Framework
Source: arXiv:1910.04708 source file (2020-02-18)
Supplement: Supplementary file 1 [file Appendix.tex]

\section{Appendix}
\label{appendix}

\subsection{NER Experiment Details}

When ali
